# Supplementary material for: Diffusiophoretic Enhancement of Mass Transfer by Nanofluids
Source: arXiv:1703.01644 source file (2017-03-05)
Supplement: Supplementary file 1 [file supp-dyenf.pdf]

# Diffusiophoretic Enhancement of Mass Transfer by Nanofluids: Supporting Information

Rakhi Dhuriya, Varun Dalia, and P. Sunthar*
*Department of Chemical Engineering, Indian Institute of Technology- Bombay, Mumbai-400076, India*

## I. THEORETICAL CALCULATION OF DIFFUSIOPHORETIC VELOCITY

The diffusiophoretic velocity of a rigid particle in a weakly non-uniform solute gradient ($a\,\nabla \ln C \ll 1$) and a thin counterion cloud ($\lambda \ll 1$) for an arbitrary zeta-potential is provided by Prieve *et al.* 1. The details of some expressions and numerical approximations carried out to obtain the final velocity are given in this section. The velocity is given by

$$U_\mathrm{p} = U_\mathrm{p}^\mathrm{c} + U_\mathrm{p}^\mathrm{e} \tag{1}$$

where, $U_\mathrm{p}^\mathrm{c}$ and $U_\mathrm{p}^\mathrm{e}$ represent the chemiophoretic and electrophoretic components of the velocity, respectively, which are further given by:

$$U_\mathrm{p}^\mathrm{c} = U_\mathrm{o}^\mathrm{c}[1 - G^\mathrm{c}\lambda]^{-1} \tag{2}$$

$$U_\mathrm{p}^\mathrm{e} = U_\mathrm{o}^\mathrm{e}[1 - G^\mathrm{e}\lambda]^{-1} \tag{3}$$

$$U_\mathrm{o}^\mathrm{c} = \frac{\varepsilon}{2\pi\eta}\left(\frac{kT}{Z\,e}\right)^2 [-\ln(1-\gamma^2)]\nabla \ln C_\infty \tag{4}$$

$$U_\mathrm{o}^\mathrm{e} = \frac{\varepsilon}{4\pi\eta}\left(\frac{kT}{Z\,e}\right)^2 \beta\bar{\zeta}\nabla \ln C_\infty \tag{5}$$

$$G^\mathrm{c} = -\frac{F_0 + \mathrm{Pe}\,(F_2 + \beta F_3)}{4\ln(1-\gamma^2)} \tag{6}$$

$$G^\mathrm{e} = \frac{F_1 + \mathrm{Pe}\,(\beta F_4 + F_5)}{2\bar{\zeta}} \tag{7}$$

where,

$$\lambda = \frac{\kappa^{-1}}{a} \tag{8}$$

$$\varepsilon \equiv 4\,\pi\,\varepsilon_0\,\varepsilon_\mathrm{r} \tag{9}$$

$$\gamma \equiv \tanh\frac{\bar{\zeta}}{4} \tag{10}$$

$$\bar{\zeta} \equiv \frac{Z\,e\,\zeta}{kT} \quad \text{(normalized zeta potential)} \tag{11}$$

$$\beta \equiv \frac{D_+ - D_-}{Z_+\,D_+ - Z_-\,D_-} \quad \text{(normalized difference in the diffusivities)} \tag{12}$$

$$\kappa \equiv \left(\frac{4\pi e^2\,Z^2\,N_\mathrm{A}\,C_\infty}{\varepsilon\,kT}\right)^{1/2} \quad \text{(inverse Debye length)} \tag{13}$$

$$\mathrm{Pe} = \frac{\varepsilon}{8\pi\eta D}\left(\frac{kT}{Z\,e}\right)^2 \tag{14}$$

$$D = \frac{(Z_+ - Z_-)D_+D_-}{Z_+D_+ - Z_-D_-}. \tag{15}$$

Here, $\varepsilon_0$ is the permittivity of free-space, $\varepsilon_\mathrm{r}$ is the relative permittivity of the medium, $\eta$ is the viscosity of the medium, $k$ is the Boltzmann constant, $T$ is the temperature, $Z$ is the valency of the ions of the assumed symmetric electrolyte, i.e. equal for positive and negative ions $Z = Z_+ = -Z_-$, $e$ is the elementary positive charge, $\zeta$ is the zeta-potential at the particle surface, $D_+$ and $D_-$ are the diffusion coefficients of the positive and negative ions respectively, $N_\mathrm{A}$ is the Avogadro number, and $C_\infty$ is the molar concentration of the solute far from the particle surface.

The functions $F_n$ used in the above calculations are complex integrals that need to be evaluated numerically. Prieve *et al.* 1 have provided tabulated numerical values of $F_n$ against the dimensionless zeta potential $\bar{\zeta}$. For convenience, we fit rational functions of the following form, taking into account the odd and even nature of the functions (caveat: the functions are least square fits in the entire range of $\bar{\zeta}$ provided, and are not

*p.sunthar@iitb.ac.in

asymptotically correct):

$$F_0 = -\bar{\zeta}^2 \left( \frac{a_0\bar{\zeta}^2 + 1}{b_0\bar{\zeta}^2 + c_0} \right), \tag{16}$$

$$F_1 = -\bar{\zeta} \left( \frac{a_1\bar{\zeta}^2 + 1}{b_1\bar{\zeta}^2 + c_1} \right), \tag{17}$$

$$F_2 = -\bar{\zeta}^4 \left( \frac{a_2\bar{\zeta}^4 + b_2\bar{\zeta}^2 + 1}{c_2\bar{\zeta}^2 + d_2} \right), \tag{18}$$

$$F_3 = -\bar{\zeta} \left( \frac{a_3\bar{\zeta}^4}{b_3\bar{\zeta}^2 + c_3} \right), \tag{19}$$

$$F_4 = -\bar{\zeta}^2 \left( \frac{a_4\bar{\zeta}^2}{b_4\bar{\zeta}^2 + c_4} \right), \tag{20}$$

$$F_5 = -\bar{\zeta} \left( \frac{a_5\bar{\zeta}^4 + b_5\bar{\zeta}^2 + 1}{c_5\bar{\zeta}^2 + d_5} \right). \tag{21}$$

The fitted parameters $P_i$ are given in the Table I.

A final note on the value of zeta potential used in the above expressions. In the present case, the bare zeta potential of the alumina nanoparticles (in the absence of dye molecules) is positive. Because of counterion (anionic fluorescein) condensation on the particle, the zeta potential $\zeta(C)$ decreases with an increase in the dye concentration $C$. The expression in Equation (1) assumes a weakly varying electrolyte (dye) concentration. However, in the initial configuration the nanoparticles at the interface are subject to a steep gradient $\nabla \ln C \sim 1/(2a)$. To be consistent with the other approximations we take the zeta potential $\zeta$ in Equation (11) to be an average of the bare value (nanofluid side of the interface without the solute) and the zeta potential at the initial electrolyte concentration (solute side of the interface)

$$\zeta_{\mathrm{av}} = \frac{\zeta(C) + \zeta(0)}{2}. \tag{22}$$

The functional dependence of $\zeta(C)$ is itself obtained by a fit of

$$\zeta = a\,C^b \tag{23}$$

to the experimental data shown in Figure 1, with $a = 0.009919$ and $b = -0.2811$, where $\zeta$ is in volts and $C$ is in mM. The bare value is given by $\zeta(0) = 0.0392$ V.

[1] D. C. Prieve, J. L. Anderson, J. P. Ebel, and M. E. Lowell, J. Fluid Mech. **148**, 247 (1984).

TABLE I: Parameters fitted to the $F_i$ functions.

| $P$ | $P_0$ | $P_1$ | $P_2$ | $P_3$ | $P_4$ | $P_5$ |
|---|---|---|---|---|---|---|
| $a$ | 0.08248 | 0.4099 | 2.645e-05 | 2055 | 0.068 | 2806 |
| $b$ | -0.002694 | -0.0023 | 0.02158 | -93.02 | -0.0006569 | 4.974e+04 |
| $c$ | 0.45 | 0.31 | -0.008695 | 2.035e+04 | 0.1 | -143.9 |
| $d$ | - | - | 2.697 | - | - | 3.112e+04 |

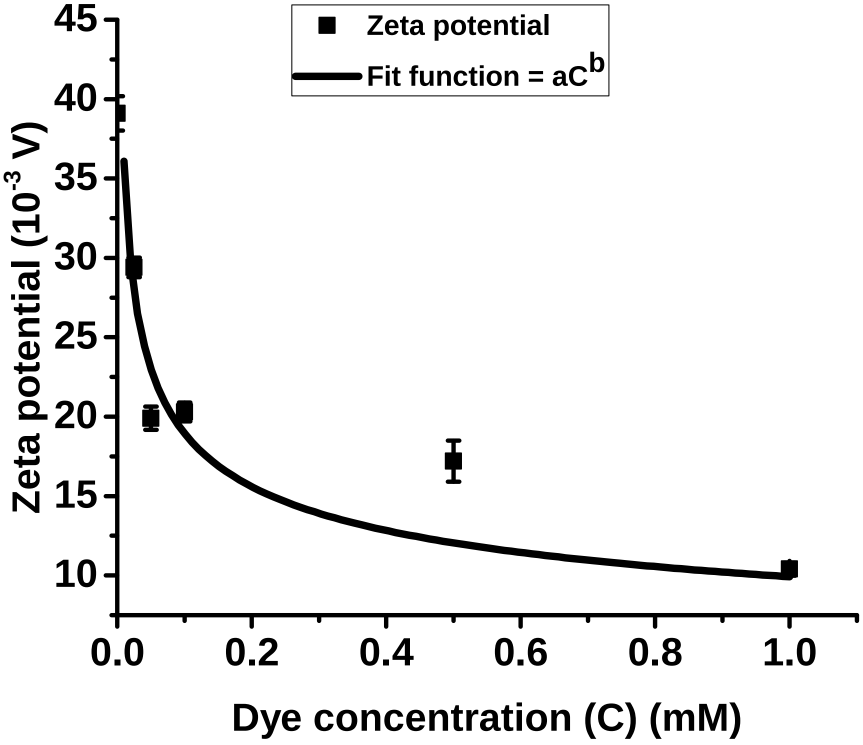


FIG. 1: Variation of the zeta potential $\zeta$ [V] of alumina nanoparticles with the concentration $C$ [mM] of uniformly surrounded fluorescein-di-sodium molecules.
